# Supplementary material for: AIRIVA: A Deep Generative Model of Adaptive Immune Repertoires
Source: arXiv:2304.13737 source file (2023-04-26)
Supplement: Supplementary file 1 [file appendix_causality_links.tex]

\section{Links to Causality}

\subsection{Disentangled Causal Process.}\label{sec:disentangled_causal_process}

%Following definition in~\cite{suter2019robustly}, \textit{disentanglement} can be defined as a property of the underlying true generation process of the data.

Consider the underlying causal process from Figure~\ref{fig:intro2}.
%; the properties of such causal process have been extensively studied in~\cite{suter2019robustly}.
Let $\mathbf{Y} = \{Y_1, \cdots, Y_K \}$ denote the observed $K$ causes of variation underlying the true data generation process. We assume there exists some confounding factors $C_1, \cdots, C_R$  on top of $\mathbf{Y}$, which results in statistical dependencies between the factors $Y_i$ and $Y_j$. The true factors of variation $\mathbf{Y}$ are \textit{elementary} in the sense that they can be changed without affecting others (there is no direct causal effect between them).

\begin{figure}[h!]
    \centering
    \begin{tikzpicture}[x=1.8cm,y=0.5cm]
        \node[latent]                              (c)      {$C$} ; %
        \node[obs, below=of c, xshift=1cm]      (y2)     {$Y_2$} ; %
        \node[obs, left=of y2]                  (y1)     {$Y_1$} ; %
        \node[obs, right=of y2]                 (yk)     {$Y_K$} ; %
        \node[obs, below=of y2]                 (x)      {$\mathbf{X}$};
        \path (y2) -- node[auto=false]{\ldots}     (yk);
        \edge {c} {y1,y2} ; %
        \edge {y1,y2,yk} {x} ; %
    \end{tikzpicture}
     \caption{\textbf{Disentangled Causal Process}: TCR repertoire $\X$ results from the combination of factors $\Y = \{Y_1, Y_2, \cdots, Y_K\}$, i.e., exposures to certain antigens, age, genetic factors, etc. which may be correlated by unobserved confounders $\mathbf{C}$. %We further assume that no factor is a parent of another.
    }
    \label{fig:intro2}
\end{figure}

Formally, a causal model for $\X$ is called \textit{disentangled}~\citep{suter2019robustly} if and only if it can be described by the causal graph of Figure~\ref{fig:intro2} and a structural causal model (SCM) of the form:
\begin{align}
    C   & \leftarrow N_c \\
    Y_k & \leftarrow f_k(\mathbf{PA}^\C_k, N_k), \mathbf{PA}^\C_k \in \{ C_1, \ldots, C_R\}, k=1, \ldots, K \\
    \X  & \leftarrow g(\Y,N_x),
\end{align}
where $N_x, N_c, N_1, \ldots, N_K$ are independent noise variables.

\subsection{Validity of counterfactuals}

\paragraph{Counterfactual generation given true causal graph}
Consider the causal graph from Figure~\ref{fig:intro2}, let $\X$ be the outcome (TCRs), $\Y$ the set of labels corresponding to the independent causes (treatments). A \textit{counterfactual} is a hypothetical observation $\X=\x^\star$ given a hypothetical treatment $Y_j=y_j^\star$ for a specific datapoint $(\x, y_j, \y_{\setminus j})$, denoted as:
\begin{equation}
    \x^\star \sim P(\X(y_j^\star) \given \X=\x, Y_j=y_j, \Y_{\setminus j}=\y_{\setminus j}).
\end{equation}
%Given a trained AIRIVA model, under which assumptions does the procedure described in Algorithm~\ref{algorithm1} generate valid counterfactuals?
Counterfactuals can be computed if we have access to the true underlying SCM, and if the modularity assumption is satisfied (i.e., interventions in the causal graph are local).
Let $\U$ refer to the set of observed and unobserved random variables in the SCM (endogenous and exogenous variables) excluding the treatment $Y_j$ and outcome $\X$. Assuming access to the true underlying SCM, we can compute valid probabilistic counterfactuals following three steps~\citep{glymour2016causal, peters2017elements}:
\begin{enumerate}
    \item \textbf{Abduction}: Use an observation $(\x,\y)$ to update the distribution of the observation-specific noise variables $\U$.
    \item \textbf{Action}: Make an intervention in the SCM, i.e., replacing the structural equation for the treatment $Y_j$ with $Y_j \defeq y_j^{\triangle}$.
    \item \textbf{Prediction}: Use the updated distribution of $\U$ from step 1 and the modified SCM from step 2 to compute the distribution of $p(\X|do(Y_j),\U)$. We can then sample a counterfactual $\x^\star \sim p(\X|do(Y_j),\U)$.
\end{enumerate}

\paragraph{Counterfactual generation given a trained AIRIVA model}
In practice, we do not know the true underlying SCM, which is why we resort to a parametrized function $f_\theta$ learned by AIRIVA to estimate the true generating process for $\X$. Counterfactuals generated by AIRIVA are valid if AIRIVA is able to recover the true structural equation $f^\star$ for $\X$ using a parametric function $f_\theta$. In such case, we can generate counterfactuals using AIRIVA following three steps:
\begin{itemize}
    \item \textbf{Abduction}: Given an  observation $\X$, sample its latent representation $\sz \sim p(\zv \given \X)$ which captures observation-specific characteristics and noise.
    \item \textbf{Action}: Replace the repertoire label value $y_j$ by an alternative label $y_j^{\triangle}$ and sample its corresponding latent factor from the conditional prior, i.e., $\sz_j^{\triangle} \sim p \left(\zv \given do(Y_j \leftarrow y^\triangle_j) \right)$.
    \item \textbf{Prediction}: Combine the latent representation from step 1 and the modified latent factor from step 2 to compute the value of $\x^\star \sim p(\X \given \sz^{\triangle})$, where $\sz^{\triangle} = [\sz_{\setminus j}, \sz_j^{\triangle}]$ is the intervened latent representation.\footnote{Without loss of generality, here we assume that we are intervening on the last factor to simplify notation.}
\end{itemize}

\paragraph{Requirements} AIRIVA will be able to recover the true data generating process if the following assumptions are satisfied:
\begin{enumerate}
    \item \textbf{Modularity assumption}: This is a standard assumption in causality which intuitively says that when we intervene on a given node $Y_j$, only the mechanism $p(Y_j|pa_j)$ should change, other mechanisms should remain unchanged~\citep{pearl2009causality}. The modularity assumption is fulfilled by construction given the graphical model of AIRIVA, since the factorized latent representation allows for local interventions in the graph.
    % AIRIVA estimates a parametric function for the SCM such that the underlying causal mechanism is modular. Indeed, if we intervene on a node $Y_j$, only the mechanism $P(Y_j|pa_j)$ changes. All other mechanisms $P(x_l|pa_l)$ remain unchanged. The intervention is local by construction.
    \item \textbf{Expressivity}: AIRIVA should be expressive enough to learn a parametrized function $f_\theta: \Y \rightarrow \X$ that corresponds to the true structural equation $f^\star$ for $\X$. This is satisfied given that we are using neural networks, which are universal approximators~\citep{hornik1989multilayer}.
    \item \textbf{Identifiability of AIRIVA's generative model}:
    %Given enough observations, we want the function learned by AIRIVA to correspond with the true structural equation $f^\star$ for $\X$.
    While unsupervised generative models have been shown to be non-identifiable~\citep{locatello2019challenging}, introducing (weak) supervision guarantees disentanglement under certain conditions~\citep{shu2019weakly}. Disentanglement in AIRIVA arises from the supervision of labels $\Y$; such labels introduce a model inductive bias towards disentanglement by adding independent per-label classification loss terms to the regularized ELBO. Indeed, \cite{shu2019weakly} shows that performing distribution matching in the augmented space of observations $\X$ and labels $\Y$ provides disentanglement guarantees on the learned representations. By performing distribution matching via maximization of the regularized ELBO in AIRIVA, we achieve approximate disentanglement, and are able to learn an approximation to the corresponding structural equations. %In other words, we can say that there exists a unique solution $f_\theta$ such that $f_\theta = f^\star$.
\end{enumerate}

\subsection{Identifiability proof for the interventional distribution $p \left(\X|do(Y_j) \right)$}\label{sec:identify}
%\TM{Are these indices correct? j, i, k, $X_i$?}
Given the causal graph from Figure~\ref{fig:intro2}, we are interested in estimating the treatment effect of an individual factor $Y_j$ on inputs $\X$. Formally, we want to compute the causal estimand $p \left(\X|do(Y_j) \right)$ given observational data. 
We assume that such causal graph follows the modularity assumption,
%We write a more formal definition of the modularity assumption below:
%
%\paragraph{Modularity Assumption.} A causal graph is said to be modular if, when we intervene on a set of nodes $\mathcal{S} \subseteq [n]$, setting them to constants, then for each node index $i$ of the causal graph, we have the following:
% \begin{enumerate}
%     \item If $i \notin \mathcal{S}$, then $p(x_i|pa_i)$ remains unchanged.
%     \item If $i \in \mathcal{S}$, then $p(x_i|pa_i)=1$ if $x_i$ is the value that $X_i$ was set to by the intervention; otherwise $p(x_i|pa_i) = 0$.
% \end{enumerate}
Let us write the observational joint distribution $p(\X,\Y)$:
\begin{align}
p \left( \X, Y_j, \Y_{\setminus j} \right) = p(\X \given Y_j, \Y_{\setminus j}) p(Y_j \given \text{pa}_j(\C)) \prod_{k \in \mathcal{S}_{\setminus j}} p(Y_k \given \text{pa}_k(\C)).
\end{align}
where $\text{pa}_j(\C)$ and $\text{pa}_k(\C)$ refer to the parents of $Y_j$ and $Y_k$ respectively. By truncated factorization and assuming modularity of the underlying causal graph, we have:
\begin{align}
    p \left(\X, \Y_{\setminus j} \given do(Y_j \leftarrow y^\triangle_j) \right) & =  p(\X \given Y_j = y^\triangle_j, \Y_{\setminus j}) \prod_{k \in \mathcal{S}_{\setminus j}} p(Y_k \given \text{pa}_k(\C)).
\end{align}
We can then marginalize out the remaining variables $Y_{\setminus j}$ as follows:
\begin{align}
    p \left(\X \given do(Y_j \leftarrow y^\triangle_j) \right) & = \int_{\Y_{\setminus j}}  p \left(\X, \Y_{\setminus j} \given do(Y_j \leftarrow y^\triangle_j) \right) d\Y_{\setminus j} \\
    & = \int_{\Y_{\setminus j}}  p(\X \given Y_j = y^\triangle_j, \Y_{\setminus j}) \prod_{k \in \mathcal{S}_{\setminus j}} p(Y_k \given \text{pa}_k(\C)) d\Y_{\setminus j} \\
    & = \mathbb{E}_{p(\Y_{\setminus j}|\C)} \left[ p \left(\X \given Y_j = y^\triangle_j, \Y_{\setminus j})  \right) \right],\label{eq:identifiability}
\end{align}
where  $p(\Y_{\setminus j}|\C)= \prod_{k \in \mathcal{S}_{\setminus j}} p(Y_k \given \text{pa}_k(\C))$. 
Given that we can write $p \left(\X|do(Y_j \leftarrow y^\triangle_j) \right)$ using observational distributions, we conclude that it is identifiable, and that the set $\Y_{\setminus j}$ is a sufficient adjustment set,\footnote{We note that, even if $\Y_{\setminus j}$ is a sufficient adjustment set, it is not necessarily the smallest one that leads to minimal variance results.} as claimed by~\cite{suter2019robustly}.

%One key property of a disentangled causal process is that the remaining components $\Y_{\setminus j}$ are a valid adjustment set to estimate the interventional effect from $Y_j$ on $\X$:
%\begin{align}
%    p(\X \,|\, do(Y_j \leftarrow y^\triangle_j})) = \mathbb{E}_{p(\mathbf{y}_{\setminus j})} \left[ p(\X \,|\, y^\triangle_j, \mathbf{y}_{\setminus j}) \right]. \label{eq:XdoY}
%\end{align}
%Because the true factors $\Y$ are observed, we can approximate the expectations in Equation~\eqref{eq:5} directly using observational data:
%\begin{align}
%   p(\X \,|\, do(Y_j \leftarrow y^\triangle_j})) \approx \frac{1}{N} \sum_{n=1}^N p(\X \,|\, y^\triangle_j, \mathbf{y}^{(n)}_{\setminus j}). \label{eq:XdoY_approx}
%\end{align}

\paragraph{Validity of Counterfactuals}\label{sec:validity_counterfactuals}
\PC{I don't think we should include this paragraph in the methods section or links to causality, its difficult to follow. We could move to Appendix though}
This procedure yields valid counterfactuals (i.e., faithful to the true underlying causal graph) if AIRIVA is able to recover the true data generation process. A first requirement is that we should observe samples from the source and target subgroups of the counterfactuals. 
%
%The key question is then: what kind of causal graphs can AIRIVA learn and do we have any guarantees to recover such graph under which conditions?
%
Underneath, AIRIVA assumes that the true underlying causal graph is a \textit{disentangled causal process}, as depicted in Figure~\ref{fig:causal}, whose defining property is that the $K$ independent factors of variation cannot cause one another~\citep{suter2019robustly}, see more details and a formal definition in Appendix~\ref{sec:disentangled_causal_process}. Indeed, labels in the generative process of AIRIVA can be changed without affecting others by construction, via sampling of the independent conditional priors in Eq.~\ref{eq:prior}. If one label causes another, generating counterfactuals by manipulating only one of the labels would break such causal relationship, yielding unrealistic counterfactuals. Although this restricts AIRIVA to a specific family of causal graphs, assuming the true causal graph to be a disentangled causal process is a reasonable assumption for several scenarios in immunomics where TCR expansion results from the combination of independent agents that do not cause each other.

\begin{figure}[]
%\begin{minipage}[b]{0.5\linewidth}
    \centering
    \caption{\textbf{Assumed causal graph}: AIRIVA assumes that data comes from a disentangled causal process, a specific family of causal graphs where the true factors of variation $Y_1, \ldots, Y_K$ cannot cause each other. Here, the observed TCR counts repertoire $\xv$ results from the combination of factors $\yv$, i.e., exposures to certain antigens, age, genetic factors, etc. which may be correlated by unobserved confounders $\cv$ but do not cause one another. %We further assume that no factor causes another.
    }\label{fig:causal}
    \begin{tikzpicture}[x=1.8cm,y=0.5cm]
        \node[latent]                              (c)      {$\cv$} ; %
        \node[latent, below=of c, xshift=1cm]      (y2)     {$Y^2$} ; %
        \node[latent, left=of y2]                  (y1)     {$Y^1$} ; %
        \node[latent, right=of y2]                 (yk)     {$Y^K$} ; %
        \node[latent, below=of y2]                 (x)      {$\xv$};
        \path (y2) -- node[auto=false]{\ldots}     (yk);
        \edge {c} {y1,y2} ; %
        \edge {y1,y2,yk} {x} ; %
    \end{tikzpicture}
    %\includegraphics[width=1.0\linewidth]{figures/causal_graph.png}
	
 % \includegraphics[width=\linewidth]{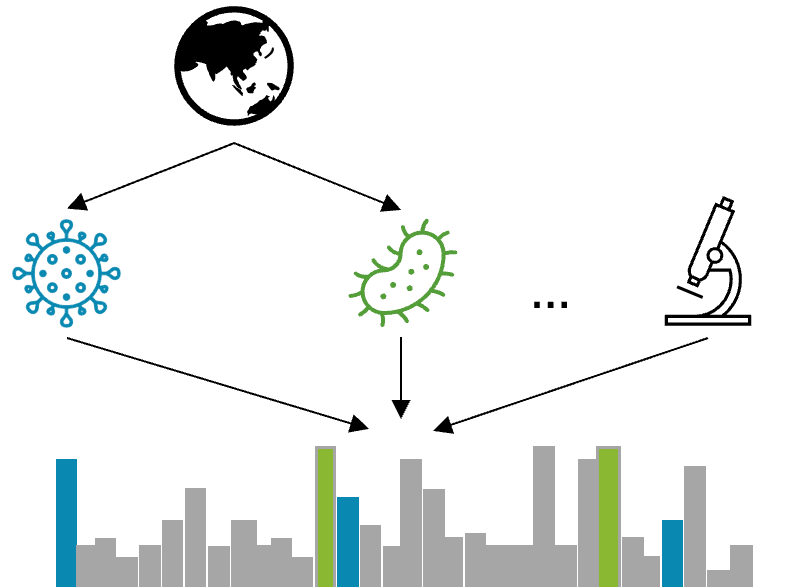}
	% \includegraphics[width=\linewidth]{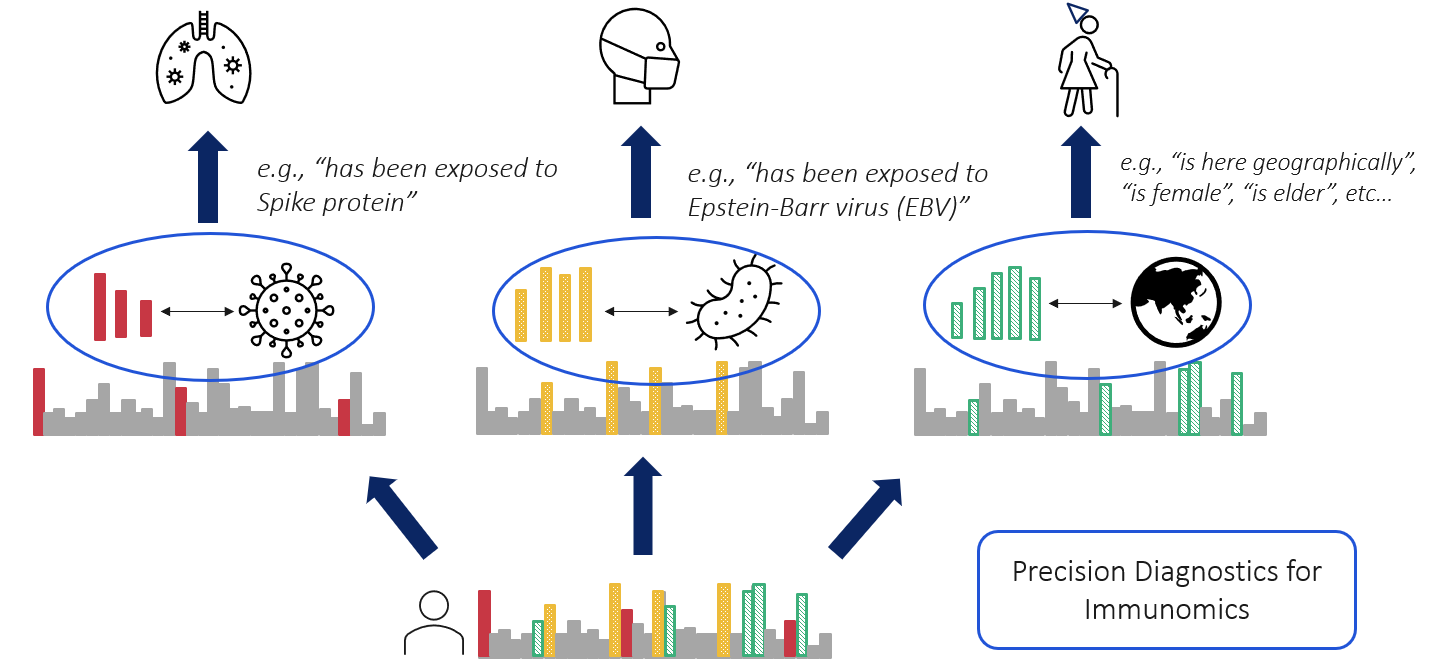}
    % \includegraphics[width=0.7\linewidth]{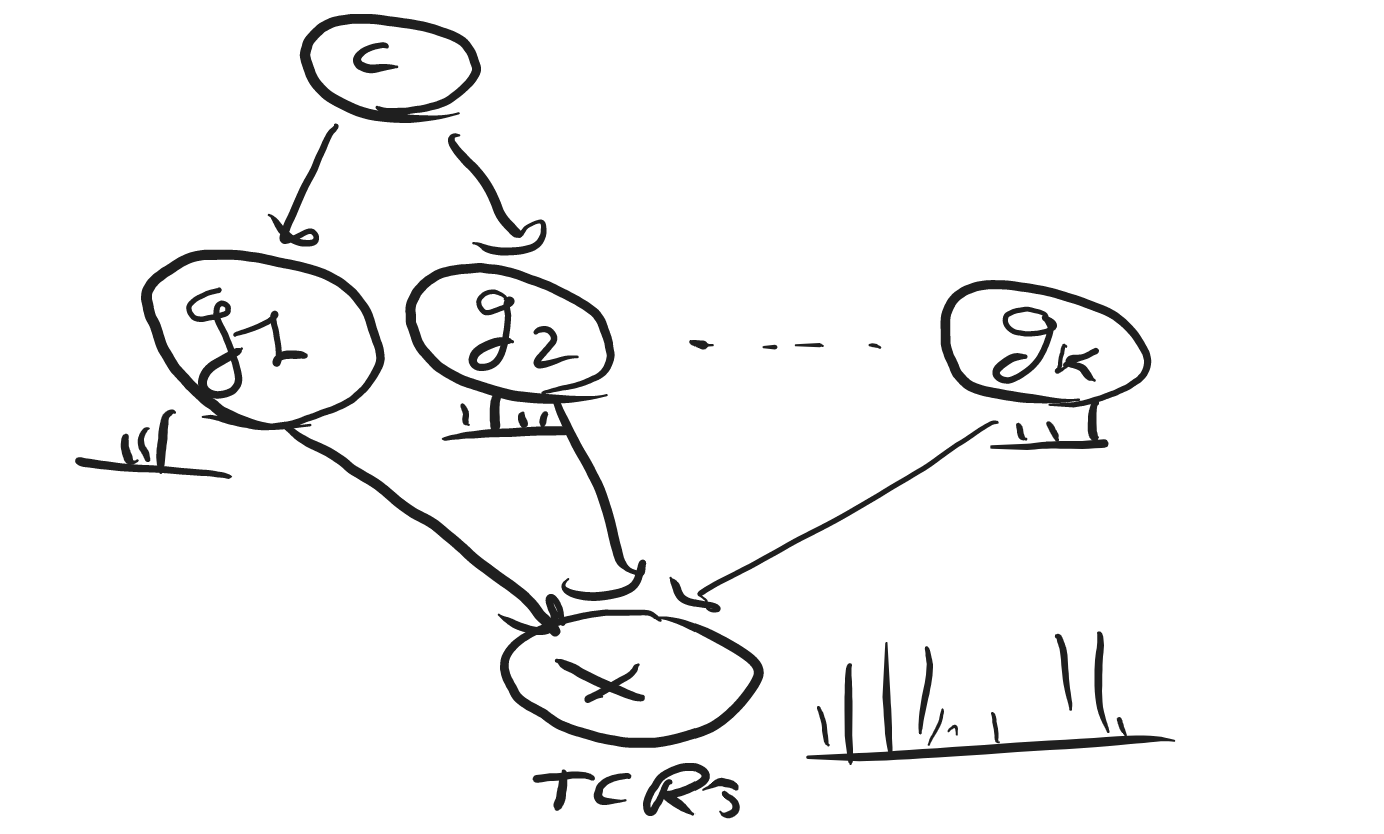}
    % \includegraphics[width=0.75\linewidth]{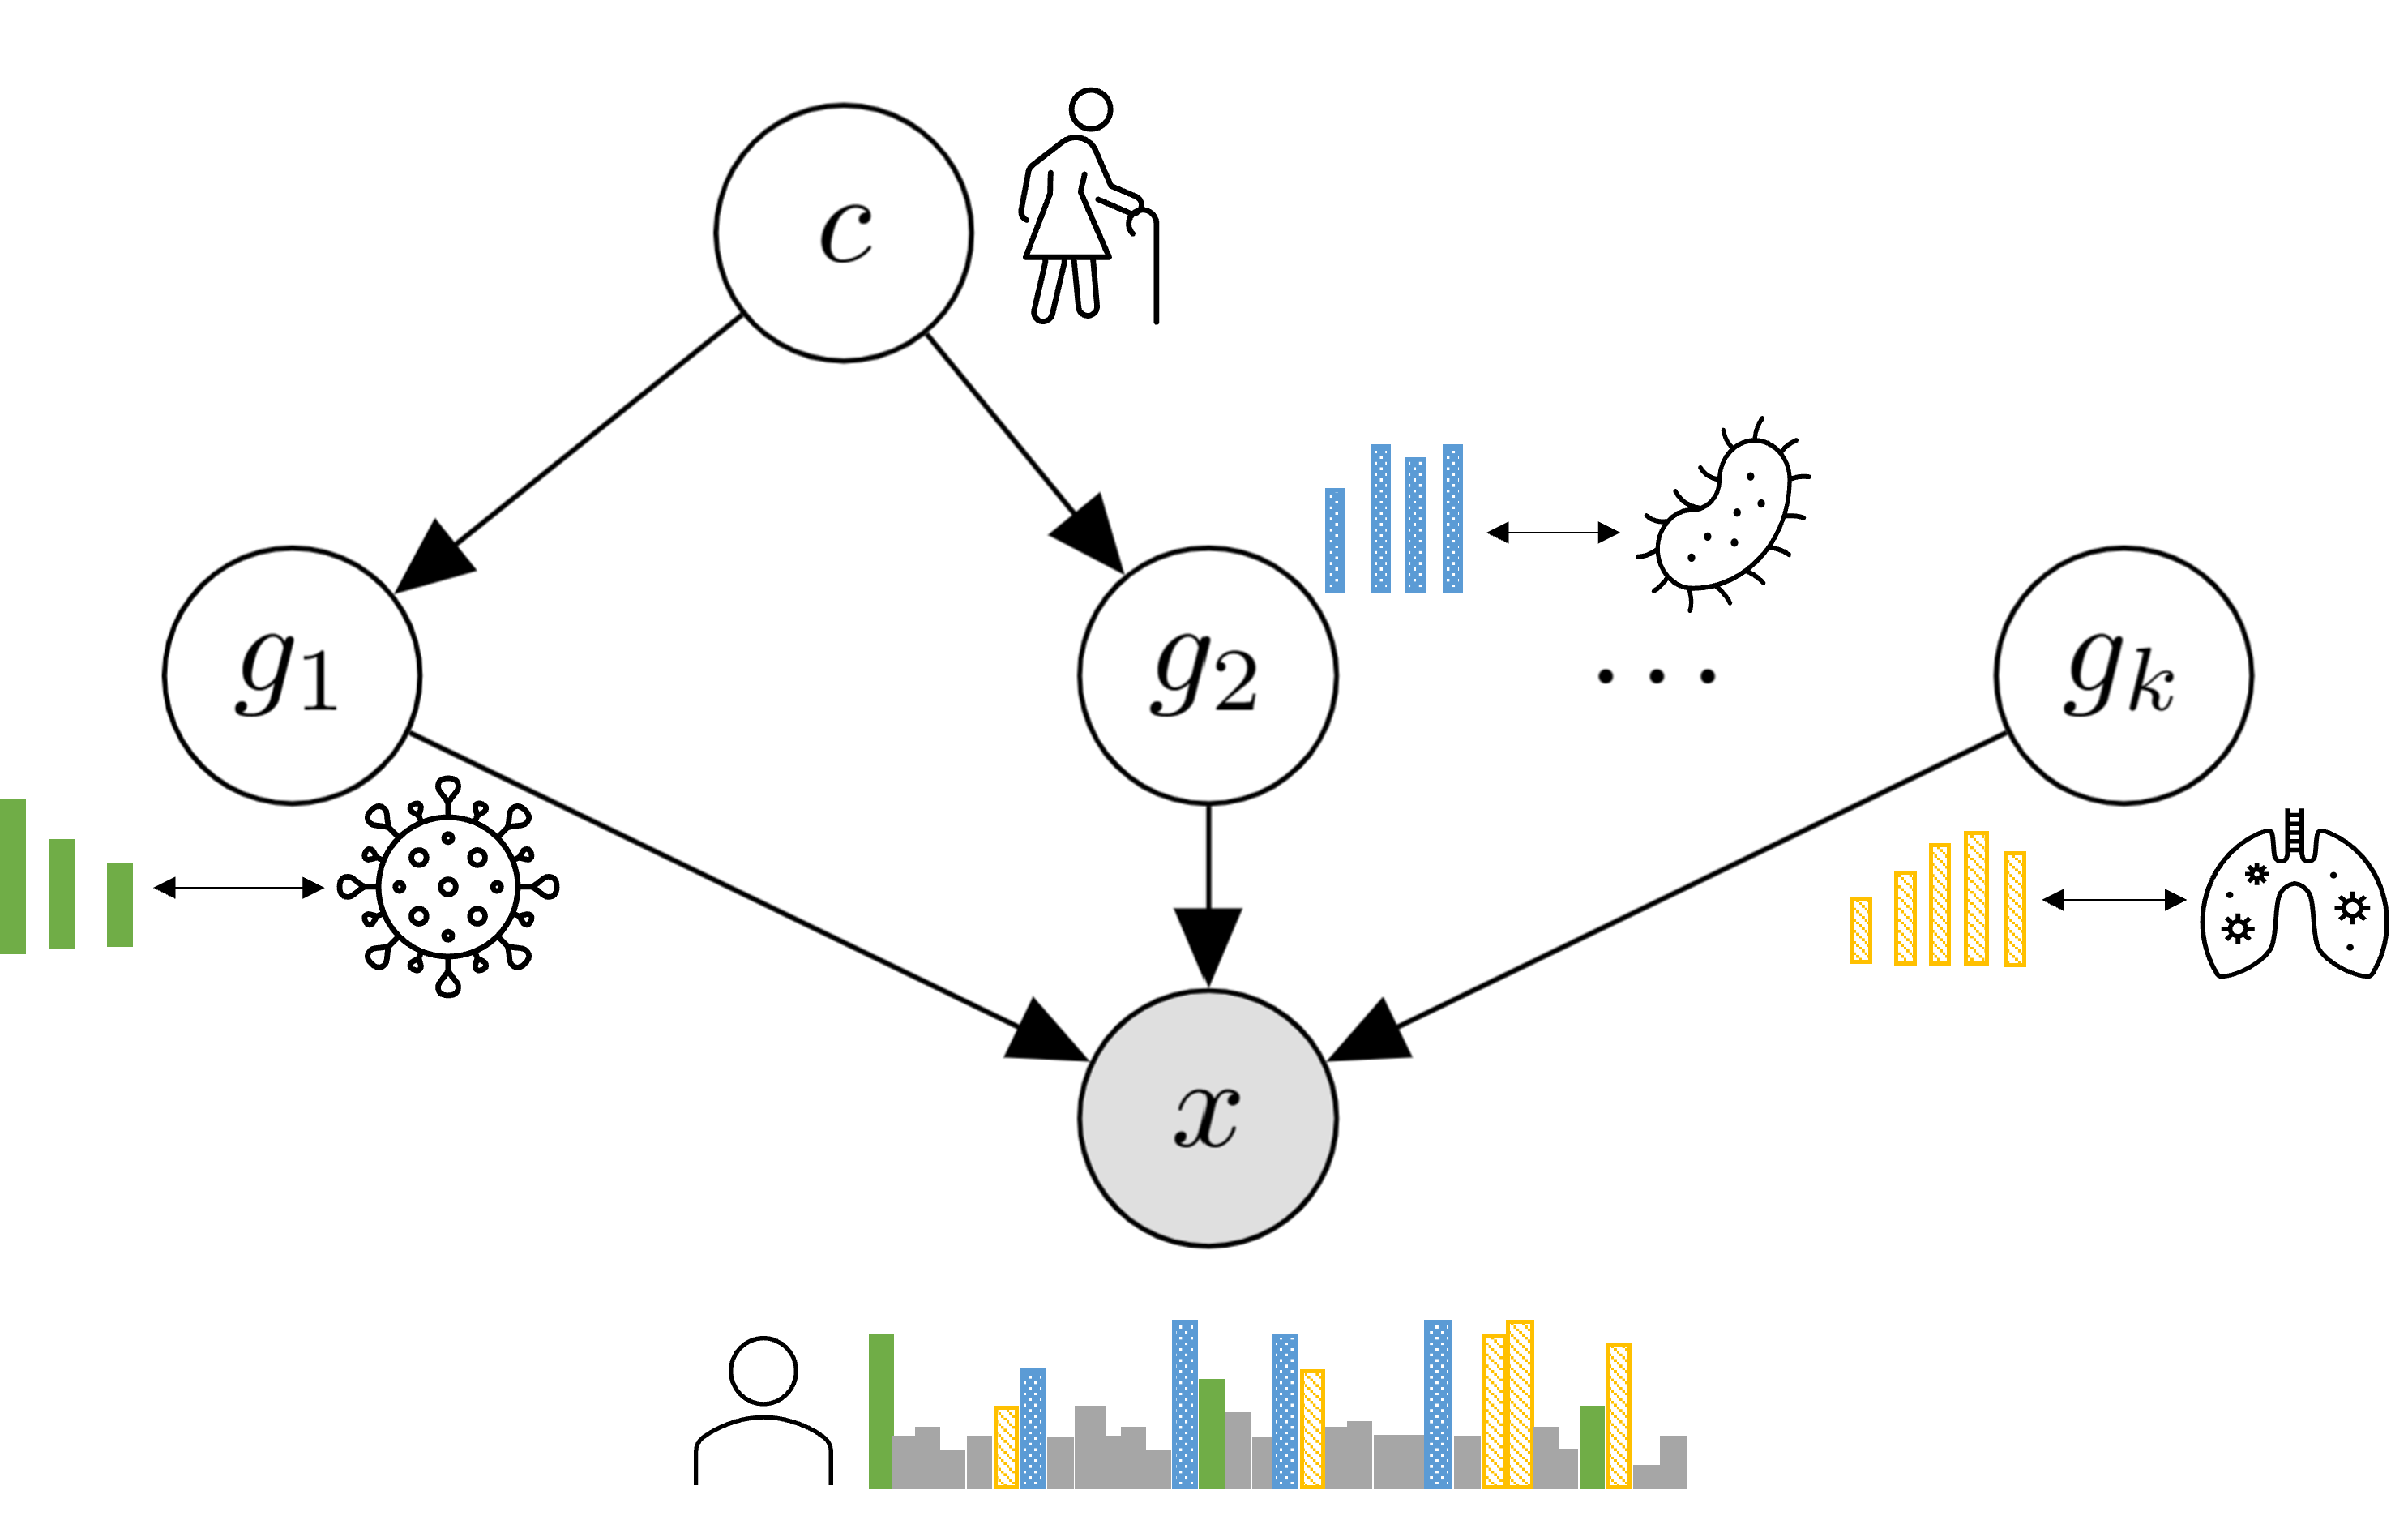}
    	% \caption{\textbf{Goal of this work}: we propose a deep generative model to decompose the adaptive immune response signal and estimate causal effects in the context of TCR count data. The inferred latent factors are human-interpretable and can be manipulated to simulate in-silico repertoires and counterfactuals, enabling downstream applications such as identification of disease-specific TCRs.
    % identify disease-specific TCRs by disentangling the TCR immune response in compositional latent factors which can be intervened on to estimate counterfactuals and causal effects. We assume the above causal graph for our data: the observed TCR counts $x$ result from a combination of elementary factors $g_1, g_2, \cdots, g_k$, which may be correlated by unobserved confounders $c$, and such that no factor is a parent of another.
%\end{minipage}
%\begin{minipage}[b]{0.5\linewidth}
%\end{minipage}
\end{figure}
