# Supplementary material for: AIRIVA: A Deep Generative Model of Adaptive Immune Repertoires
Source: arXiv:2304.13737 source file (2023-04-26)
Supplement: Supplementary file 2 [file OLD_appendix.tex]

% PLOTS TO ADD
% - TCR counts for factual data (to compare for validation of conditional generation
% - 


% \begin{figure*}[h!]
% 	\centering
% 	\begin{subfigure}{0.49\textwidth}
% 		%\includegraphics[width=\linewidth]{figures/covid/coutnerfactuals_best.png}
%         \includegraphics[width=\linewidth]{figures/hsv12/best_run/counterfactuals1.png}
% 	\caption{Posterior samples $z \sim q(z|x)$}
% 	\end{subfigure}
%         \hfill
% 	\begin{subfigure}{0.49\textwidth}
% 		\includegraphics[width=\linewidth]{figures/hsv12/best_run/counterfactuals2.png}
% 		\caption{Posterior predictive $q(y|x)$}
% 	\end{subfigure}       
% 	\caption{\textbf{Counterfactual generation with AIRIVA for the HSV dataset}. (left) Latent representation $¦zv \sim q(\zv|\xv)$ for factual data (first column) and counterfactual data (columns 2-5) stratified by subgroups. (right) Posterior predictive distribution $q(\yv|\xv)$ for factual (first column) and counterfactual data (columns 2-5) stratified by subgroups.
% 	}
% 	\label{fig:counterfactuals_hsv}
% \end{figure*}

% \begin{figure*}[h!]
% 	\centering
%         \includegraphics[width=\textwidth]{figures/hsv12/best_run/ates_hsv.png}
%         %\includegraphics[width=\textwidth]{figures/hsv12/best_run/correct_ATE_HSV.png}
% 	\caption{\textbf{Estimation of Treatment Effects for HSV dataset.} by (left) Naive approach: splitting all available individuals into cases and controls for each positive label, regardless of any unobserved confounder, using AIRIVA to impute the potential outcomes and estimate average treatment effects via (middle) conditional generation or (right) counterfactuals. For this dataset, we do not have wetlab data for validation.}
%  %In this example, we estimate the effect of the spike antigen by taking all vaccinated individuals, and compute their corresponding counterfactual of removing the effect of vaccine.}
% 	\label{fig:figure_ATEs_hsv}
% \end{figure*}

\paragraph{Summary.}
In this technical note, we tackle the following research questions:
\begin{enumerate}
    \item Is the causal estimand $p(\X|do(Y_j))$ identifiable, i.e., can we express such causal quantity using statistical quantities?
    \item Under which assumptions does a trained AIRIVA model generate valid counterfactuals?
    %\begin{enumerate}
    %    \item Given the causal process from Figure~\ref{fig:intro} and the structural equations $f^\star: \Y \rightarrow \X$, is AIRIVA flexible enough to learn a parametric function $f_\theta$ such that $f_\theta \equiv f^\star$?
    %    \item Is the generative model of AIRIVA identifiable? Given an infinite number of observations, is the solution unique?
    %\end{enumerate}
\end{enumerate}

Next section defines the notion of disentangled causal process, a central concept to answer these questions.

\subsection{Disentangled Causal Process.}

%Following definition in~\cite{suter2019robustly}, \textit{disentanglement} can be defined as a property of the underlying true generation process of the data.

Consider the underlying causal process from Figure~\ref{fig:intro2}.
%; the properties of such causal process have been extensively studied in~\cite{suter2019robustly}.
Let $\mathbf{Y} = \{Y_1, \cdots, Y_K \}$ denote the observed $K$ causes of variation underlying the true data generation process. We assume there exists some confounding factors $C_1, \cdots, C_R$  on top of $\mathbf{Y}$, which results in statistical dependencies between latent factors $Y_i$ and $Y_j$. The true factors of variation $\mathbf{Y}$ are \textit{elementary} in the sense that they can be changed without affecting others (there is no direct causal effect between them).

\begin{figure}[h!]
    \centering
    \begin{tikzpicture}[x=1.8cm,y=0.5cm]
        \node[latent]                              (c)      {$C$} ; %
        \node[obs, below=of c, xshift=1cm]      (y2)     {$Y_2$} ; %
        \node[obs, left=of y2]                  (y1)     {$Y_1$} ; %
        \node[obs, right=of y2]                 (yk)     {$Y_K$} ; %
        \node[obs, below=of y2]                 (x)      {$\mathbf{X}$};
        \path (y2) -- node[auto=false]{\ldots}     (yk);
        \edge {c} {y1,y2} ; %
        \edge {y1,y2,yk} {x} ; %
    \end{tikzpicture}
     \caption{\textbf{Disentangled Causal Process}: TCR repertoire $\X$ results from the combination of factors $\Y = \{Y_1, Y_2, \cdots, Y_K\}$, i.e., exposures to certain antigens, age, genetic factors, etc. which may be correlated by unobserved confounders $\mathbf{C}$. %We further assume that no factor is a parent of another.
    }
    \label{fig:intro2}
\end{figure}

Formally, a causal model for $\X$ is called \textit{disentangled} if and only if it can be described by the causal graph of Figure~\ref{fig:intro2} and a structural causal model (SCM) of the form:
\begin{align}
    C   & \leftarrow N_c \\
    Y_i & \leftarrow f_i(\mathbf{PA}^\C_i, N_i), \mathbf{PA}^\C_i \in \{ C_1, \ldots, C_R\}, i=1, \ldots, K \\
    \X  & \leftarrow g(\Y,N_x),
\end{align}
where $N_x, N_c, N_1, \ldots, N_k$ are independent noise variables.







\subsection{Identifiability proof for $p \left(\X|do(Y_j) \right)$}\label{sec:identify}

Given the causal graph from Figure~\ref{fig:intro2}, we are interested in estimating the treatment effect of an individual factor $Y_j$ on inputs $\X$. Formally, we want to compute the causal estimand $p \left(\X|do(Y_j) \right)$ given observational data. 
%
We assume that such causal graph follows the modularity assumption, this is a standard assumption in causality which intuitively says that when we intervene on a given node $X_i$, then only the mechanism $P(x_i|pa_i)$ should change, other mechanisms remain unchanged~\cite{pearl2009causality}. We write a more formal definition of the modularity assumption below:

\paragraph{Modularity Assumption.} A causal graph is said to be modular if, when we intervene on a set of nodes $\mathcal{S} \subseteq [n]$, setting them to constants, then for each node index $i$ of the causal graph, we have the following:
\begin{enumerate}
    \item If $i \notin \mathcal{S}$, then $p(x_i|pa_i)$ remains unchanged.
    \item If $i \in \mathcal{S}$, then $p(x_i|pa_i)=1$ if $x_i$ is the value that $X_i$ was set to by the intervention; otherwise $p(x_i|pa_i) = 0$.
\end{enumerate}
Let us write the observational joint distribution $p(\X,\Y)$:
\begin{align}
p \left( \X, Y_j, \Y_{\setminus j} \right) = p(\X \given Y_j, \Y_{\setminus j}) p(Y_j \given \text{pa}_j(\C)) \prod_{k \in \mathcal{S}_{\setminus j}} p(Y_k \given \text{pa}_k(\C)).
\end{align}
where $\text{pa}_j(\C)$ and $\text{pa}_k(\C)$ refer to the parents of $Y_j$ and $Y_k$ respectively. By truncated factorization and assuming modularity of the underlying causal graph~\cite{pearl2009causality}, we have:
\begin{align}
    p \left(\X, \Y_{\setminus j} \given do(Y_j \leftarrow y^\triangle_j) \right) & =  p(\X \given Y_j = y^\triangle_j, \Y_{\setminus j}) \prod_{k \in \mathcal{S}_{\setminus j}} p(Y_k \given \text{pa}_k(\C)).
\end{align}
We can then marginalize out the remaining variables $Y_{\setminus j}$ as follows:
\begin{align}
    p \left(\X \given do(Y_j \leftarrow y^\triangle_j) \right) & = \int_{\Y_{\setminus j}}  p \left(\X, \Y_{\setminus j} \given do(Y_j \leftarrow y^\triangle_j) \right) d\Y_{\setminus j} \\
    & = \int_{\Y_{\setminus j}}  p(\X \given Y_j = y^\triangle_j, \Y_{\setminus j}) \prod_{k \in \mathcal{S}_{\setminus j}} p(Y_k \given \text{pa}_k(\C)) d\Y_{\setminus j} \\
    & = \mathbb{E}_{p(\Y_{\setminus j}|\C)} \left[ p \left(\X \given Y_j = y^\triangle_j, \Y_{\setminus j})  \right) \right],\label{eq:identifiability}
\end{align}
where  $p(\Y_{\setminus j}|\C)= \prod_{k \in \mathcal{S}_{\setminus j}} p(Y_k \given \text{pa}_k(\C))$. 
Given that we can write the quantity $p \left(\X|do(Y_j \leftarrow y^\triangle_j) \right)$ using observational distributions, we conclude that it is identifiable, and that the set $\Y_{\setminus j}$ is a sufficient adjustment set, as claimed by~\cite{suter2019robustly}.

%One key property of a disentangled causal process is that the remaining components $\Y_{\setminus j}$ are a valid adjustment set to estimate the interventional effect from $Y_j$ on $\X$:
%\begin{align}
%    p(\X \,|\, do(Y_j \leftarrow y^\triangle_j})) = \mathbb{E}_{p(\mathbf{y}_{\setminus j})} \left[ p(\X \,|\, y^\triangle_j, \mathbf{y}_{\setminus j}) \right]. \label{eq:XdoY}
%\end{align}
%Because the true factors $\Y$ are observed, we can approximate the expectations in Equation~\eqref{eq:5} directly using observational data:
%\begin{align}
%   p(\X \,|\, do(Y_j \leftarrow y^\triangle_j})) \approx \frac{1}{N} \sum_{n=1}^N p(\X \,|\, y^\triangle_j, \mathbf{y}^{(n)}_{\setminus j}). \label{eq:XdoY_approx}
%\end{align}

\subsection{Validity of Counterfactuals}

\paragraph{Counterfactual generation given true causal graph}
Consider the causal graph from Figure~\ref{fig:intro2}. Let $\X$ be the outcome (TCRs), $\Y$ the set of labels corresponding to the independent causes (treatments). A \textit{counterfactual} is a hypothetical observation $\X=\x^\star$ given a hypothetical treatment $Y_j=y_j^\star$ for a specific datapoint $(\x, y_j, \y_{\setminus j})$, denoted as:
\begin{equation}
    \x^\star \sim P(\X(y_j^\star) \given \X=\x, Y_j=y_j, \Y_{\setminus j}=\y_{\setminus j}).
\end{equation}
%Given a trained AIRIVA model, under which assumptions does the procedure described in Algorithm~\ref{algorithm1} generate valid counterfactuals?
Counterfactuals can be computed if we have access to the true underlying structural causal model (SCM), and if the modularity assumption is satisfied (i.e., interventions in the causal graph are local).
Let $\U$ refer to the set of observed and unobserved random variables in the SCM (endogenous and exogenous variables) excluding the treatment $Y_j$ and outcome $\X$. Assuming access to the true underlying SCM, we can compute valid probabilistic counterfactuals following three steps~\cite{glymour2016causal, peters2017elements}:
\begin{enumerate}
    \item \textbf{Abduction}: Use an observation $(\x,\y)$ to update the distribution of the observation-specific noise variables $\U$.
    \item \textbf{Action}: Make an intervention in the SCM, i.e., replacing the structural equation for the treatment $Y_j$ with $Y_j \defeq y_j^{\triangle}$.
    \item \textbf{Prediction}: Use the updated distribution of $\U$ from step 1 and the modified SCM from step 2 to compute the distribution of $p(\X|do(Y_j),\U)$. We can then sample a counterfactual $\x^\star \sim p(\X|do(Y_j),\U)$.
\end{enumerate}

\paragraph{Counterfactual generation given a trained AIRIVA model}
In practice, we do not know the true underlying SCM, which is why we resort to a parametrized function $f_\theta$ learned by AIRIVA to estimate the true structural equation for $\X$. Counterfactuals generated by AIRIVA are valid if AIRIVA is able to recover the true structural equation $f^\star$ for $\X$ using a parametric function $f_\theta$. In such case, we can generate counterfactuals using AIRIVA following three steps (see Algorithm~\ref{alg:ctf} for details):
\begin{itemize}
    \item \textbf{Abduction}: Given an  observation, compute the distribution of the latent space $\sz$, which is a proxy for the intrinsic noise U, for a given individual (determine value of intrinsic noise U, that gives us the indivudalized SCM for that particular observation).
    \item \textbf{Action}: Modify the SCM, by replacing the repertoire label $y_j$ by an alternative label $y_j^\star$.
    \item \textbf{Prediction}: Use the value of U from step 1 and the modified SCM from step 2 to compute the value of $X(t)$.
\end{itemize}

To demonstrate that counterfactuals generated by AIRIVA are valid, we need to prove:
\begin{enumerate}
    \item \textbf{Modularity assumption}: the modularity assumption is fulfilled given the graphical model of AIRIVA (this is trivial, since the factorized latent representation allows for local interventions in the graph by construction).
    \item \textbf{Expressivity}: AIRIVA is expressive enough to learn a parametrized function $f_\theta: \Y \rightarrow \X$ that corresponds to the true structural equation $f^\star$ for $\X$, i.e., $f_\theta = f^\star$ (this is also trivial given that we are using neural networks, which are universal approximators~\cite{hornik1989multilayer}).
    \item \textbf{Identifiability}: Given an infinite number of observations, the function learned by AIRIVA converges to the true structural equation $f^\star$ for $\X$. In other words, we can say that there exists a unique solution $f_\theta$ such that $f_\theta = f^\star$.
\end{enumerate}
\textbf{Side-question}: does the correct computation of counterfactuals require the structural equation from $\Y$ to $\X$ to be an invertible function? If two different label combinations $y_1$ and $y_2$ might yield the same observation $\x$, then we cannot recover with certainty what was the label assignment for that particular observation. Having said that, I believe we can compute a probability of counterfactuals accounting for such uncertainty in label assignments.

%Implications include: reconstruction error close to zero, high predictive performance of counterfactuals, high disentanglement score. 

\paragraph{Modularity assumption under AIRIVA.} AIRIVA estimates a parametric function for the SCM such that the underlying causal mechanism is modular. Indeed, if we intervene on a node $Y_j$, only the mechanism $P(Y_j|pa_j)$ changes. All other mechanisms $P(x_l|pa_l)$ remain unchanged. The intervention is local by construction.

\paragraph{Expressivity.} Is AIRIVA expressive enough to recover the true SCM function $f^\star$ of a disentangled causal process?
Given that we have access to observations for $\Y$, the only function that we need to learn using AIRIVA is $g: \Y \rightarrow \X$. Given that neural networks are universal function approximators~\cite{hornik1989multilayer}, we conclude that AIRIVA has enough expressivity to learn any mapping function~$g$.

\paragraph{Identifiability of AIRIVA's generative model.} 
%Given an infinite amount of data, is the solution unique, i.e., $f_\theta=f^\star$?
%
%Assumption: every factor of variation is exactly recoverable from the observation $\X$, i.e., $e(g(S)) = S$.
While unsupervised generative models have been shown to be non-identifiable~\cite{locatello2019challenging}, introducing (weak) supervision has been shown to be enough to guarantee disentanglement~\cite{shu2019weakly}. Disentanglement in AIRIVA arises from the supervision of labels $\Y$; such labels introduce a model inductive bias towards disentanglement by adding independent per-label classification loss terms to the regularized ELBO. Indeed, \cite{shu2019weakly} shows that performing distribution matching in the augmented space of observations $\X$ and labels $\Y$ provide disentanglement guarantees on the learned representations. By performing distribution matching via maximization of the regularized ELBO in AIRIVA, we achieve disentanglement~\cite{shu2019weakly} and are able to learn the structural equations of an SCM that follows the causal graph from Figure~\ref{fig:intro}.
% Disentanglement in AIRIVA arises from the supervision of labels $\Y$ and the model inductive biases (by making the per-label classifiers independent.$

\begin{figure}[ht!]
	\centering
    \begin{tikzpicture}[x=1.5cm,y=0.7cm]
        \node[obs, xshift=-1cm]                   (yns)     {$Y_1$} ; %
        \node[obs, right=of yns, xshift=-0.6cm]                  (ys)      {$Y_2$} ; %
        \node[obs, right=of ys]                   (yd)      {$Y_K$} ; %
        \path (ys) -- node[auto=false]{\ldots} (yd);
        \node[latent, below=of yns]               (zns)     {$Z_1$} ; %
        \node[latent, right=of zns, xshift=-0.6cm]               (zs)      {$Z_2$} ; %
        \node[latent, right=of zs]                (zk)      {$Z_K$} ; %
        \path (zs) -- node[auto=false]{\ldots} (zk);
        \node[latent, right=of zk]                (zx)      {$Z_\epsilon$} ; %
        \node[obs, below=of zs, xshift=1.1cm]     (x)       {$\X$} ; %
        %\edge {dis} {yns,ys} ; %
        %\edge {lab} {yns,ys,yk} ; %
        \edge {yns} {zns} ; %
        \edge {ys} {zs} ; %
        \edge {yd} {zk} ; %
        \edge {zns,zs,zk,zx} {x} ; %
    \end{tikzpicture}
    \caption{Probabilistic graphical model. Nodes $Y^1$ to $Y^K$ are the same observed labels as depicted in the underlying causal graph from Figure~\ref{fig:intro2}.}
    \label{fig:airiva-pgm}
\end{figure}

\section{Appendix 2: Details on Datasets, Training and Model Selection}

\subsection{Further Details on the Datasets}

\paragraph{HSV}
Our dataset consists of 1003 repertoires with 451 HSV-1 only positives, 74 HSV-2 only positives, 223 samples that are positive for both and 255 that are positive for neither. We split our data 80:20 for model training and validation. In addition we have a holdout set of 241 samples only used for evaluation. We filter TCRs by a one-sided FET as described above for each binary label down to a p-value threshold of 3e-4. This gives us a total set of 325 sequences. Because of the overlapping binary labels we expect these sequences to be a mix of HSV-1 specific, HSV-2 specific and shared TCRs. 
%Can decide whether to include this or not:
%A logistic growth enhanced sequence model (cite Greissl) trained naively on each label independent of the other shows reasonable performance for both HSV-1 and HSV-2 (0.76 %AUROC and 0.8 AUROC respectively) but upon closer inspection is not able to separate the two labels. For example, the HSV-1 model performance drops to AUROC of 0.56 for samples %that are also HSV-2 positive.

\paragraph{COVID-19}
This dataset comprises immune repertoires from a total of 7152 individuals in the training set and 5131 in the holdout set. Of those in the training cohort, 1954 have been positively diagnosed with a natural COVID-19 infection, 477 are healthy controls that have been vaccinated, and the remaining 5198 are unvaccinated healthy controls. Of those in the holdout cohort, 525 are PCR-positive for COVID-19, 400 have been fully vaccinated with one of the previously mentioned COVID-19 vaccines and have not had previous COVID-19 infection, 4606 are unvaccinated controls sampled prior to the COVID-19 pandemic (December 2020), and the remaining 100 are vaccinated individuals that are PCR-positive for COVID-19. Figure~\ref{fig:covid_data_structure} shows the underlying structure of the COVID-19 dataset.

\begin{figure}[h!]
	\centering
 %\includegraphics[width=\linewidth]{figures/final/mira_covid.png}
 %\includegraphics[width=\linewidth]{figures/final/ates.png}
		\includegraphics[width=0.3\textwidth]{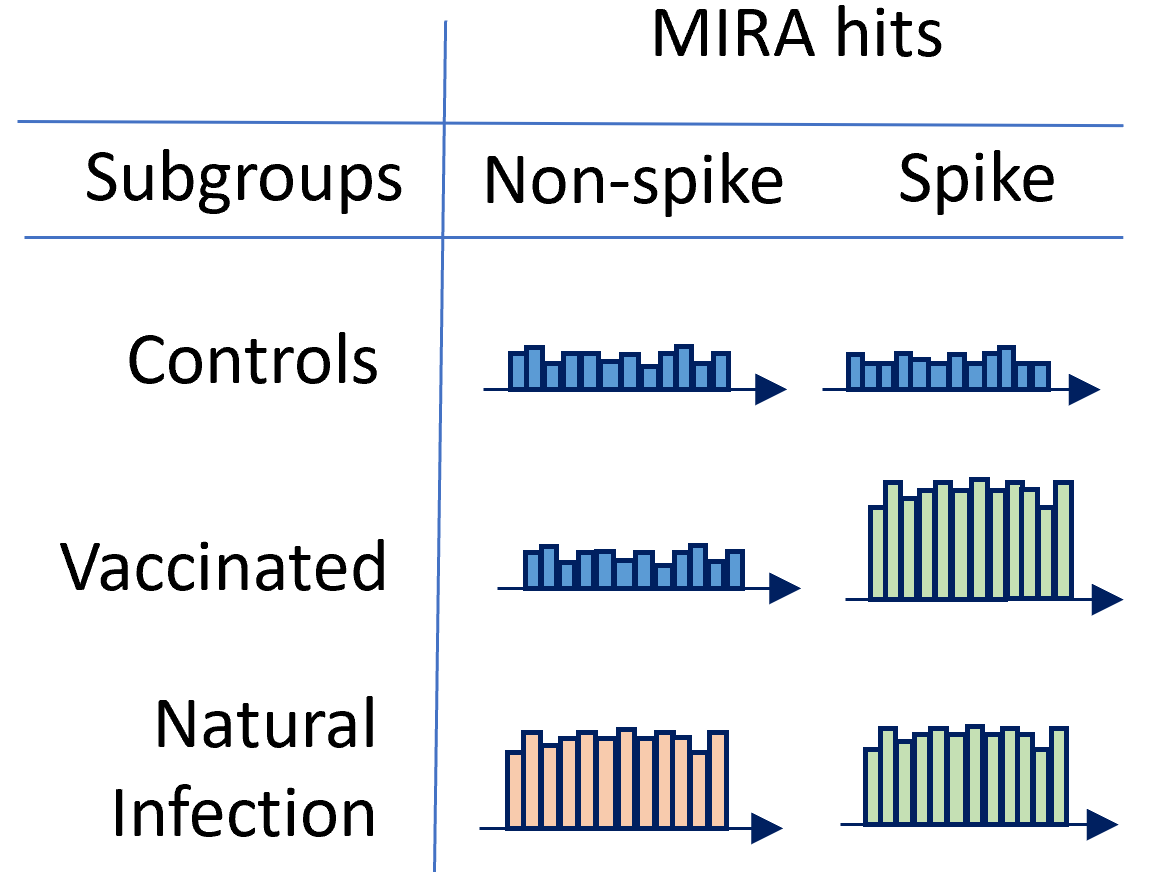}
		\caption{Underlying data structure for COVID-19.}
		\label{fig:covid_data_structure}
\end{figure}

% %Train
% %Num vaccinated: 477/7152
% %Num cases: 1954/7152
% %Num controls: 5198/7152
% % Holdout
% %Num vaccinated: 400/5131
% %Num cases: 525/5131
% %Num controls: 4606/5131

\subsection{Further Details on the Baselines}

\paragraph{Naive Group Mean Difference} The naive GMD corresponds to the associational difference between the observed cases and controls, without any adjustment in the remaining covariate set. In particular:
\begin{equation}
    \text{Naive-GMD}(Y_j) = \mathbb{E}[X \given  Y_j = 1] - \mathbb{E}[X \given Y_j = 0]
\end{equation}

\paragraph{Matched Group Mean Difference} The matched GMD w.r.t label $Y_j$ corresponds to the associational difference between the observed case and control groups conditioning on the other covariates $\Y_{\setminus j}$ being identical, i.e.:
\begin{equation}
    \text{Matched-GMD}(Y_j|\Y_{\setminus j}=\boldsymbol{y}^{\triangle}_{\setminus j}) = \mathbb{E}[X \given  Y_j = 1, \Y_{\setminus j}=\boldsymbol{y}^{\triangle}_{\setminus j}] - \mathbb{E}[X \given Y_j = 0, \Y_{\setminus j}=\boldsymbol{y}^{\triangle}_{\setminus j}].
\end{equation}
Note that we can condition on different values $\boldsymbol{y}^{\triangle}_{\setminus j}$ to match cases and controls. Concretely, in the case of COVID-19, we compute $\text{Matched-GMD}(Y_\text{nonspike} \given Y_\text{spike}=1, Y_\text{depth}=\bar{y}_{\text{depth}})$ (difference in expectation between covid-positive and vaccinated repertoires) and $\text{Matched-GMD}(Y_\text{spike} \given Y_\text{nonspike}=0, Y_\text{depth}=\bar{y}_{\text{depth}})$ (difference in expectation between vaccinated and healthy repertoires).
%\begin{equation}
%    \text{Matched-GMD}(Y_\text{NS} \given Y_\text{S}=1} = \mathbb{E}[X \given  Y_j = 1, \Y_{\setminus j}=\boldsymbol{y}^{\triangle}_{\setminus j}] - \mathbb{E}[X \given Y_j = 0, \Y_{\setminus j}=\boldsymbol{y}^{\triangle}_{\setminus j}].
%\end{equation}



\subsection{Further Details on Experimental Setup}




\subsection{Additional Results}


\begin{figure}[h!]
	\centering
 %\includegraphics[width=\linewidth]{figures/condgen/stem_control.png}
 %\includegraphics[width=\linewidth]{figures/condgen/stem_vaccinated.png}
 %\includegraphics[width=\linewidth]{figures/condgen/stem_covid.png}
  \includegraphics[width=\linewidth]{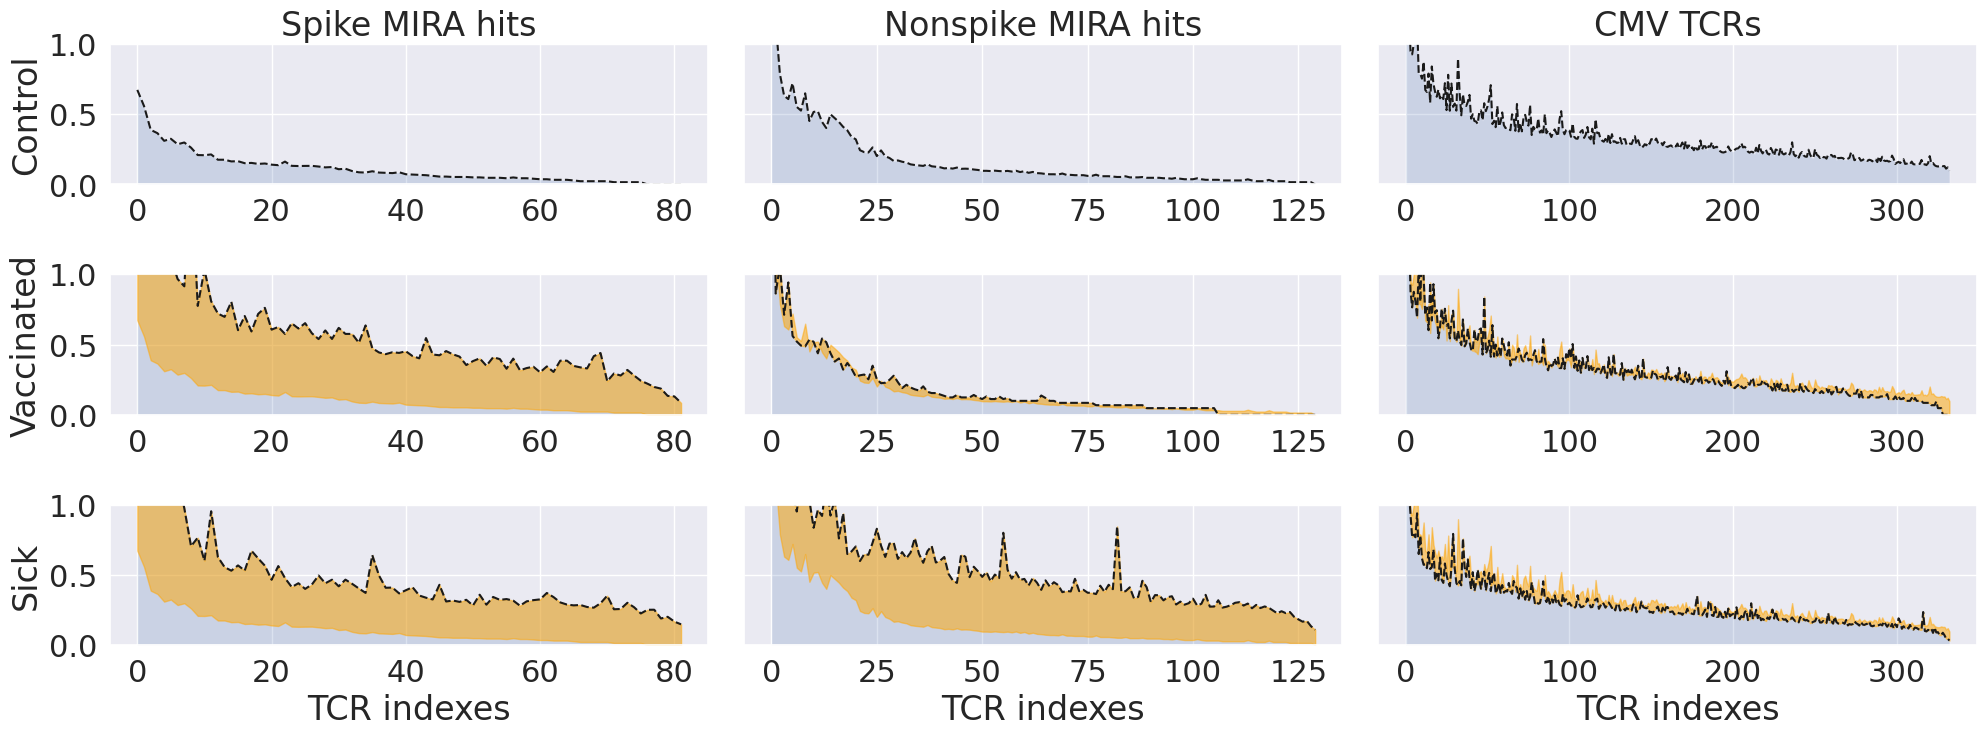}
	\caption{\textbf{TCR counts in factual data.} TCR counts sorted by magnitude of estimated Poisson rate for \textbf{factual data} in the train set, splitted by type of MIRA hit in 3 groups: spike-specific, nonspike-specific, or COVID-unrelated TCRs.
	}
\end{figure}

% \begin{figure}[h!]
% 	\centering
%   \includegraphics[width=\linewidth]{figures/final/best_run/mira_counts_cond_gen2.png}
% 	\caption{TCR counts sorted by magnitude of estimated Poisson rate for factual data, splitted by type of MIRA hit in 3 groups: spike-specific, nonspike-specific, or COVID-unrelated TCRs. See corresponding plots for factual data in Appendix.
% 	}
% \end{figure}



%   \paragraph{Classification of MIRA hits} In order to quantitatively assess the quality of learnt TCR associations, we use the ATEs from generated counterfactuals as a score to rank TCR specificity with respect to spike and non-spike proteins respectively, and evaluate against ground truth MIRA hits. Figure~\ref{fig:ppv_vs_fdr} shows the positive predictive value (PPV), based on the true MIRA TCRs recovered for that protein, and false discovery rate (FDR), using MIRA hits for the other class of protein, when selecting the top-$k$ TCRs as ranked by spike and non-spike ATEs. In order to make our metrics robust against the choice of the threshold $k$, we compute integrated metrics for $k$ taking all values between 10 and 100. We report average metrics across 5 trained AIRIVA models.
 
%  We compare the ATEs estimated by AIRIVA with empirical ATEs by group mean difference in a naive and matched setting. Both the naive setting and AIRIVA rely on all available data for treatment effect estimation, but we can see that both conditional and counterfactual ATEs from AIRIVA significantly outperform naive group mean differences with respect to both PPV and FDR, approaching the performance of the matched setting for spike MIRA, with counterfactuals outperforming for non-spike MIRA. %Further Figures reporting the FDR w.r.t to the CMV-specific TCRs can be found in the Appendix.
 
%  \begin{figure}[t!]
% 	\centering
% 	%\includegraphics[width=0.45\linewidth]{figures/final/ppv_mira1.png}
%     %\includegraphics[width=0.45\linewidth]{figures/final/ppv_mira2.png}
%  \includegraphics[width=\linewidth]{figures/final/best_run/mira_classification_avg_5runs.png}
% 	\caption{\textbf{Label-specific TCR classification}. We compare the ATEs estimated using AIRIVA against group mean differences in a naive and matched setting.
% 	}
% 	\label{fig:ppv_vs_fdr}
% \end{figure}

% \subsection{Counterfactual Generation}

% %The model, that by itself is a useful tool to interpret the data, also provides a meachanism to generate realistic counterfactuals. These synthetically generated data allows us to use the model as a \emph{data driven simulator for immunomics}.

% Next, we assess AIRIVA's capacity to generate counterfactuals by intervening on the labels, as described in Section~\ref{sec:counterfactuals}. Figure~\ref{fig:counterfactuals}a shows the latent space representation of the observed data (first column), and counterfactuals (other columns) transformed from one subgroup to another. Figure~\ref{fig:counterfactuals}b shows the corresponding posterior predictive distribution $q(\yv|\xv) = \int q(\yv|\zv)q(\zv|\xv)d\zv$ for factuals and counterfactuals.
% %
% Both figures show that we can generate counterfactuals by manipulating specific labels. We note that the last column corresponds to a repertoire subgroup that can never been seen in reality: these are out-of-distribution counterfactuals. Interestingly, although AIRIVA is not supposed to handle those correctly without further inductive biases, it manages to learn the right direction of variation in the latent space.

% \begin{figure*}[h!]
% 	\centering
% 	\begin{subfigure}{0.45\textwidth}
% 		%\includegraphics[width=\linewidth]{figures/covid/coutnerfactuals_best.png}
%         \includegraphics[width=\linewidth]{figures/final/best_run/counterfactuals_all_stochastic1b.png}
% 		\caption{Posterior samples $\sz \sim q(\zv|\xv)$ for COVID-19}
% 	\end{subfigure}
%         \hfill
% 	\begin{subfigure}{0.53\textwidth}
% 		\includegraphics[width=\linewidth]{figures/final/best_run/counterfactuals_all_stochastic2b.png}
% 		\caption{Posterior predictive $q(\yv|\xv)$ for COVID-19}
% 	\end{subfigure}
 
%  \vspace{0.3cm}
 
%  \begin{subfigure}{0.49\textwidth}
%         \includegraphics[width=\linewidth]{figures/hsv12/best_run/counterfactuals1.png}
% 	\caption{Posterior samples $\sz \sim q(\zv|\xv)$ for HSV}
% 	\end{subfigure}
%         \hfill
% 	\begin{subfigure}{0.49\textwidth}
% 		\includegraphics[width=\linewidth]{figures/hsv12/best_run/counterfactuals2.png}
% 		\caption{Posterior predictive $q(\yv|\xv)$ for HSV}
% 	\end{subfigure}
% 	\caption{\textbf{Counterfactual generation with AIRIVA}. (left) Latent representation $\sz \sim q(\zv|\xv)$ for factual data (first column) and counterfactual data (other columns) stratified by subgroups. (right) Posterior predictive distribution $q(\yv|\xv)$ for factual (first column) and counterfactual data (columns 2-5) stratified by subgroups. The labels assignment is: control = [0 0], hsv2 [0 1], hsv1 [1 0], hsv1+hsv2 [1 1].
%     %The ``nonspike only'' subgroup can never be observed in reality. %Similar plots for HSV dataset can be found in Figure~\ref{fig:counterfactuals_hsv} of the Appendix.
% 	}
% 	\label{fig:counterfactuals}
% \end{figure*}


\begin{figure}[h!]
\centering
\begin{minipage}{0.65\textwidth}
    \centering
%\begin{subfigure}
    \includegraphics[width=\linewidth]{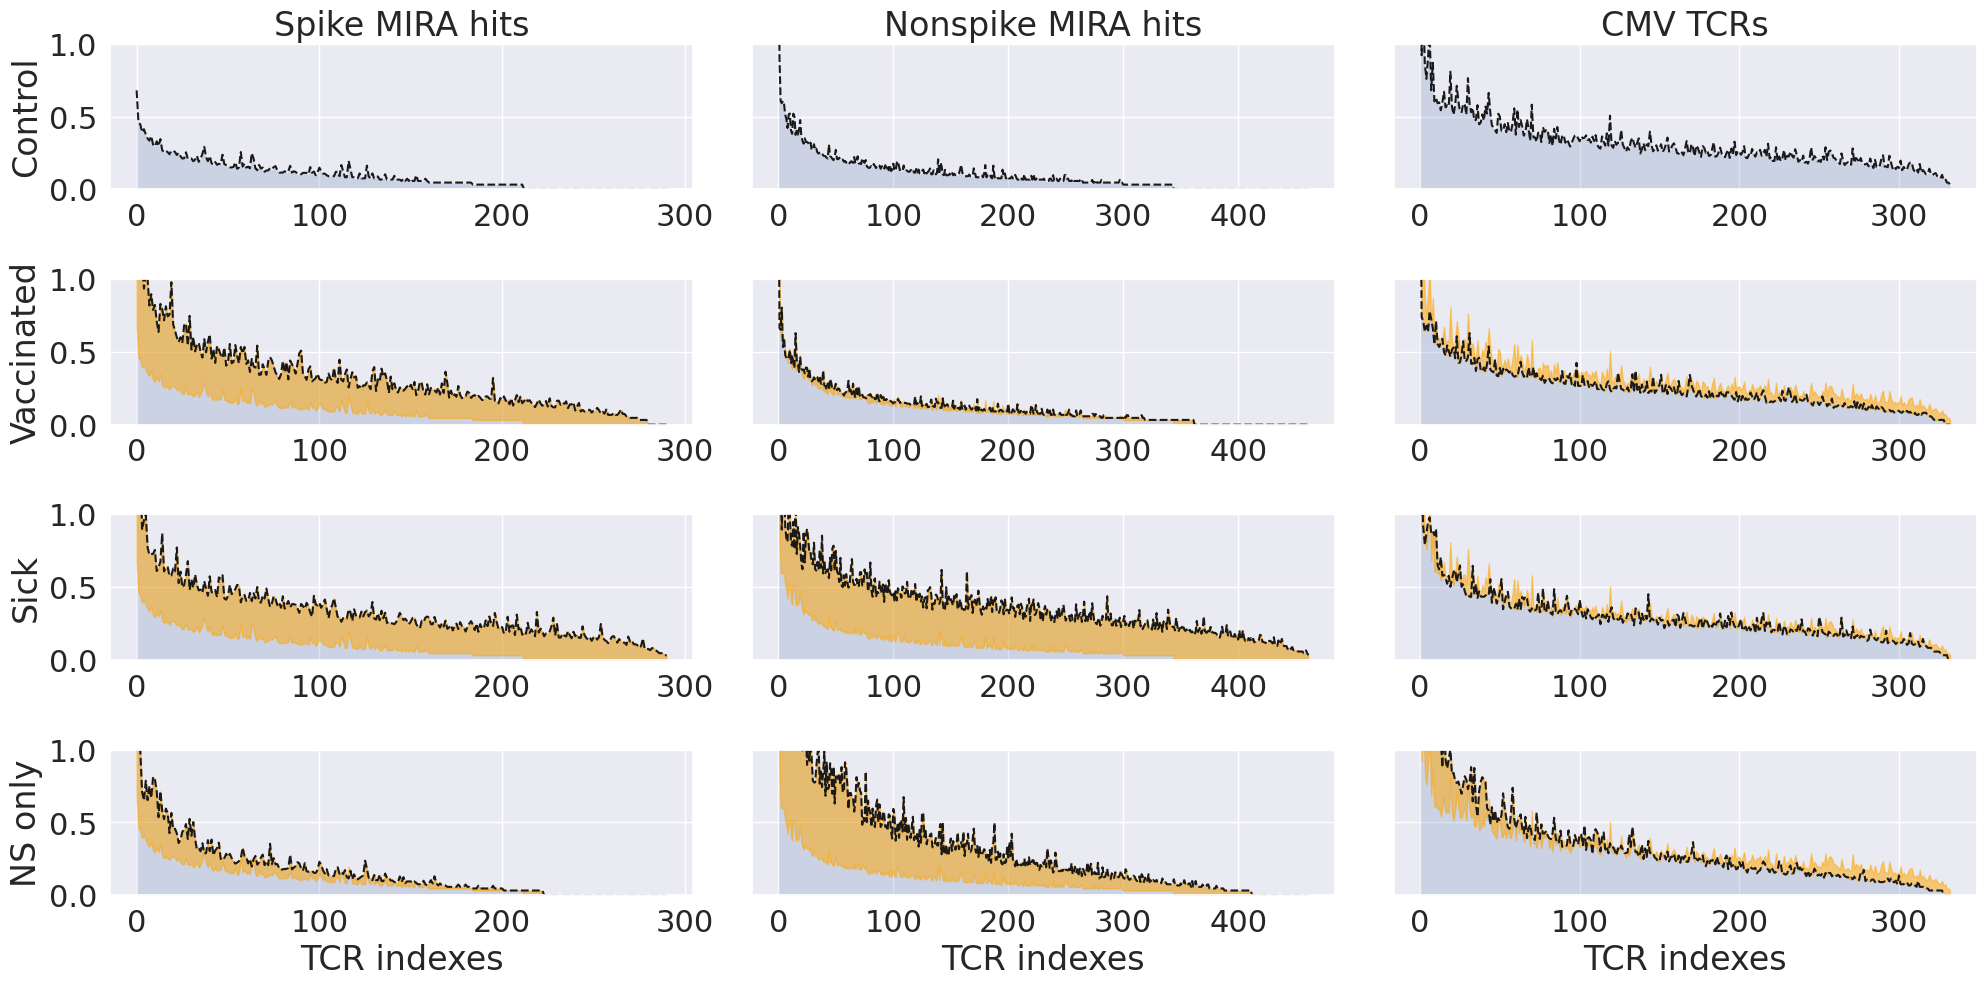}
    % \includegraphics[width=\linewidth]
    % {figures/final/airiva_mira_counts.png}
    \subcaption{(a) Intervening on binary labels}
    %\subcaption{(a) Average number of TCR counts in the input space}
    \label{fig:binary}
    \vspace{0.4cm}
%\end{subfigure}
%\begin{subfigure}
    %\includegraphics[width=\linewidth]{figures/final/heatmap_decoder2.png}
    %\includegraphics[width=\linewidth]{figures/final/best_run/decoder_heatmap.png}
    %\subcaption{(b) Average decoder Poisson rate in the latent space}
    %\label{fig:decoder_heatmap}
%\end{subfigure}
\end{minipage}
\hfill
\begin{minipage}{0.31\textwidth}
    \centering
%\begin{subfigure}
    %\includegraphics[width=\linewidth]{figures/final/depth_intervention.png}
    \includegraphics[width=\linewidth]{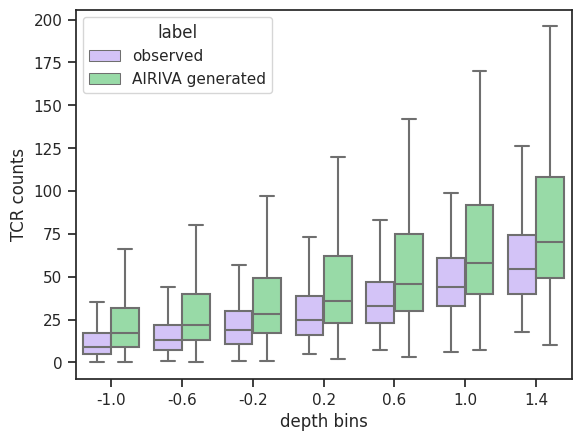}
	\subcaption{(b) Intervening on depth}
	\label{fig:effect_interven_depth}
%\end{subfigure}
\end{minipage}
\caption{\textbf{Conditional generation with AIRIVA}. (a) Mean activation per TCR in input space (in decreasing order), where activation corresponds to the average of TCR counts across repertoires plus one standard deviation. 
%\TM{Not enough description to undertand the figure.  Needs to be crystal clear in text or here.  What is the take awya?}
(b) Decoder Poisson rate averaged across different types of TCR mapped to the latent space.
(c) Distribution of TCR counts on factual and in-silico data.
%See corresponding plots for factual data in Appendix.
 }\label{fig:cond_generationBIS}
\end{figure}


Figure~\ref{fig:decoder_heatmap} illustrates the Poisson rates splitted by the same TCR subsets when sweeping over coordinates in the latent subspace ($\sz_\text{nonspike}$, $\sz_\text{spike}$). We can see that, for spike MIRA hits, the decoder is able to learn decision boundaries that are orthogonal to $\sz_\text{spike}$. For the nonspike TCRs however, we find that the decision boundary is warped in the lower right nonspike-only region of the space. This is expected, as the region for which we have no data in observed repertoires and the decoder has no information to learn an orthogonal boundary without further inductive biases in the out-of-distribution region. The activation for CMV annotations remain mostly inactive in the latent spike/nonspike subspace, highlighting AIRIVA's capacity to disentangle different underlying signals.

%\TM{Not enough info for reader} 
Finally, Figure~\ref{fig:effect_interven_depth} compares the distribution of total sum of TCR counts for conditionally generated in-silico repertoires against the empirical distribution when stratifying by depth. Although the in-silico repertoires tend to exhibit a higher number of outliers due to the assumed Poisson distribution, the marginal distribution of in-silico repertoires follows the same trend than the empirical one, enabling us to control depth in a realistic manner.


\paragraph{Faithful Counterfactual Generation for COVID-19}

The model, that by itself is a useful tool to interpret the data, also provides a meachanism to generate realistic counterfactuals. These synthetically generated data are used for model selection as described in Subsection~\ref{sec:exp-setup}, and allows us to use the model as a \emph{data driven simulator for immunomics}. AIRIVA generates counterfactuals by intervening on the labels, as described in Section~\ref{sec:counterfactuals}. Figure~\ref{fig:counterfactuals}(a) shows the latent space representation of the observed data (first column), and counterfactuals (other columns) transformed from one subgroup to another. Figure~\ref{fig:counterfactuals}(b) shows the corresponding posterior predictive distribution $q(\yv|\xv) = \int q(\yv|\zv)q(\zv|\xv)d\zv$ for factuals and counterfactuals.
%
Both figures show that we can generate counterfactuals by manipulating specific labels. We note that the last column corresponds to a repertoire subgroup that can never been seen in reality: these are out-of-distribution counterfactuals. Interestingly, although AIRIVA is not supposed to handle those correctly without further inductive biases, it manages to learn the right direction of variation in the latent space.

\begin{figure}[]
    \begin{minipage}{0.95\textwidth}
        \centering
	%\begin{subfigure}{0.45\textwidth}
		%\includegraphics[width=\linewidth]{figures/covid/coutnerfactuals_best.png}
        %\includegraphics[width=\linewidth]{figures/final/best_run/counterfactuals_all_stochastic1b.png}
        \includegraphics[width=\linewidth]{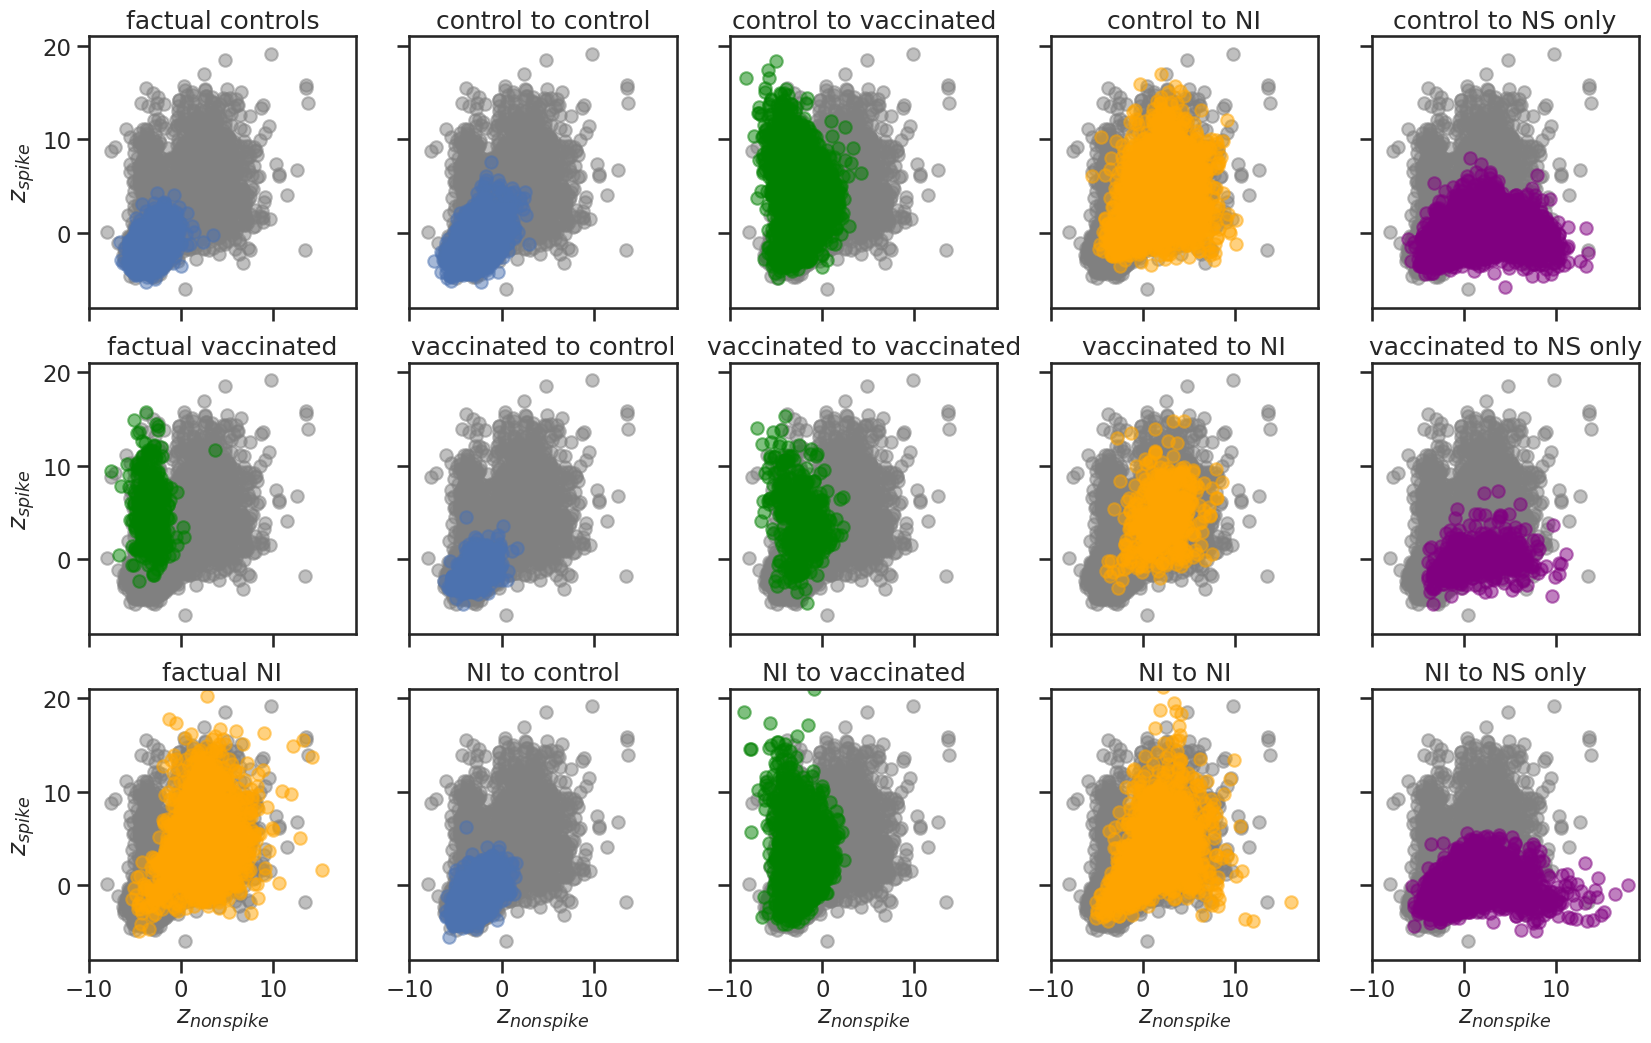}
		\subcaption{(a) Posterior samples $\sz \sim q(\zv|\xv)$}
	%\end{subfigure}
    \end{minipage}
    \begin{minipage}{0.95\textwidth}
        \centering
	%\begin{subfigure}{0.53\textwidth}
	%\includegraphics[width=\linewidth]{figures/final/best_run/counterfactuals_all_stochastic2b.png}
     \includegraphics[width=\linewidth]{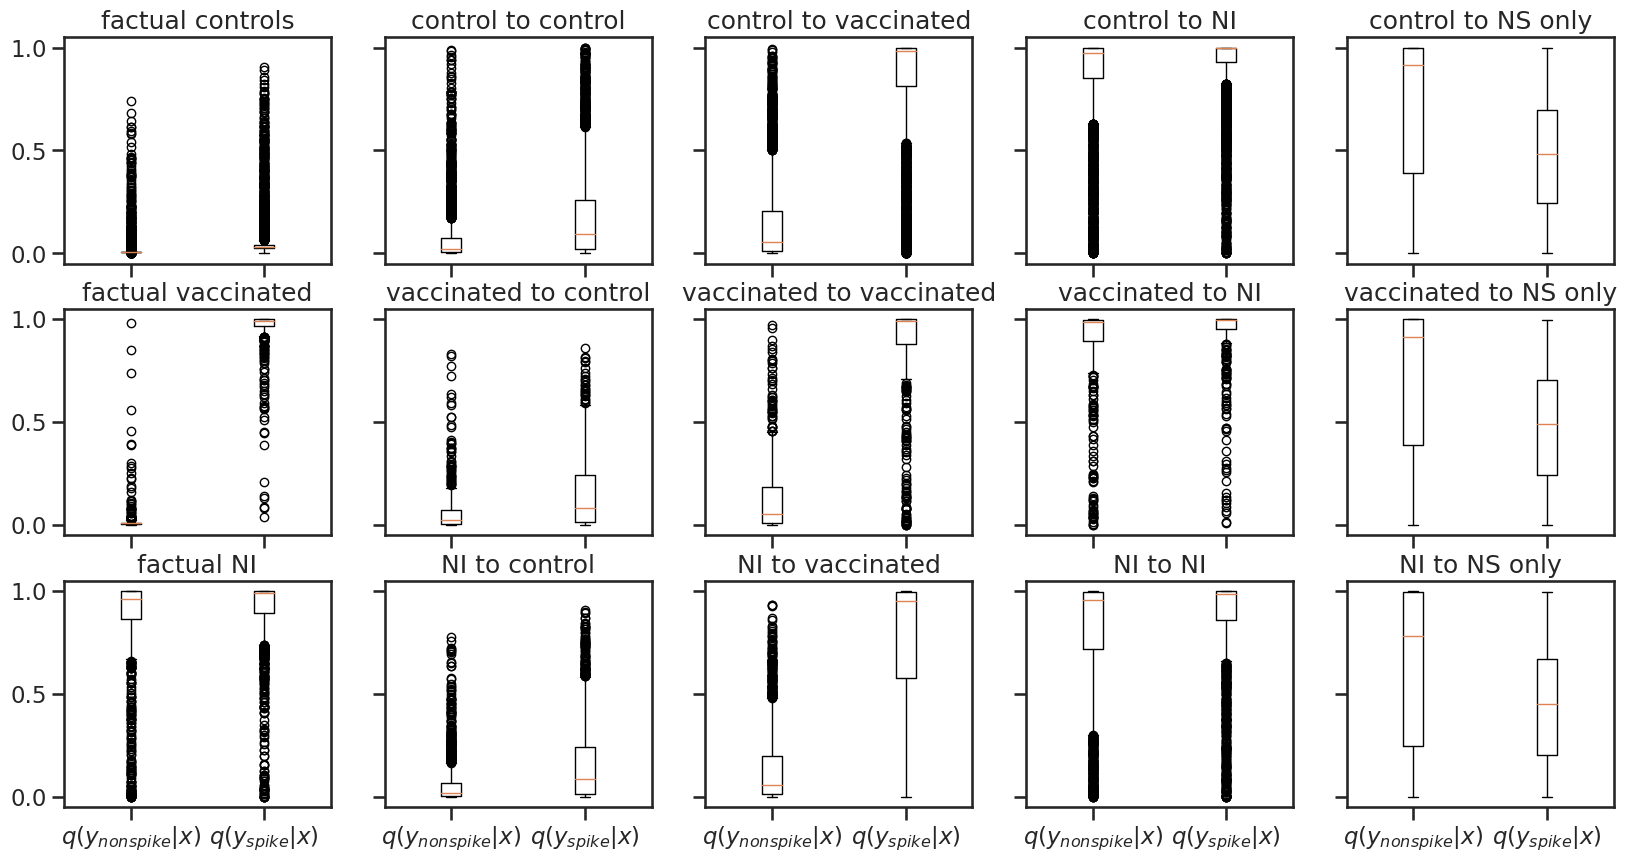}
		\subcaption{(b) Posterior predictive $\y \sim q(\yv|\xv)$}
	%\end{subfigure}
    \end{minipage}
	\caption{\textbf{Counterfactual generation for COVID-19}. (a) Latent representation $\sz \sim q(\zv|\xv)$ for factual data (first column) and counterfactual data (other columns) stratified by subgroups. (b) Posterior predictive distribution $q(\yv|\xv)$ for factual (first column) and counterfactual data (columns 2-5) stratified by subgroups. The labels assignment is: control = [0 0], natural infection [1 0], and vaccinated repertoires [0 1]. The ``nonspike only'' subgroup can never be observed in reality. \MFP{Report quantitative metric, CF-AUCROC.} %Similar plots for HSV dataset can be found in Figure~\ref{fig:counterfactuals_hsv} of the Appendix.
	}
	\label{fig:counterfactuals}
\end{figure}


\begin{figure}[h!]
	\centering
	\begin{minipage}{0.44\textwidth}
		%\includegraphics[width=\textwidth]{figures/latent_space/fig1a_annotated}
        %\includegraphics[width=\textwidth]{figures/covid/latent_covid_best.png}
        %\includegraphics[width=\textwidth]{figures/hsv12/best_run/latent_train.png}
        \includegraphics[width=\textwidth]{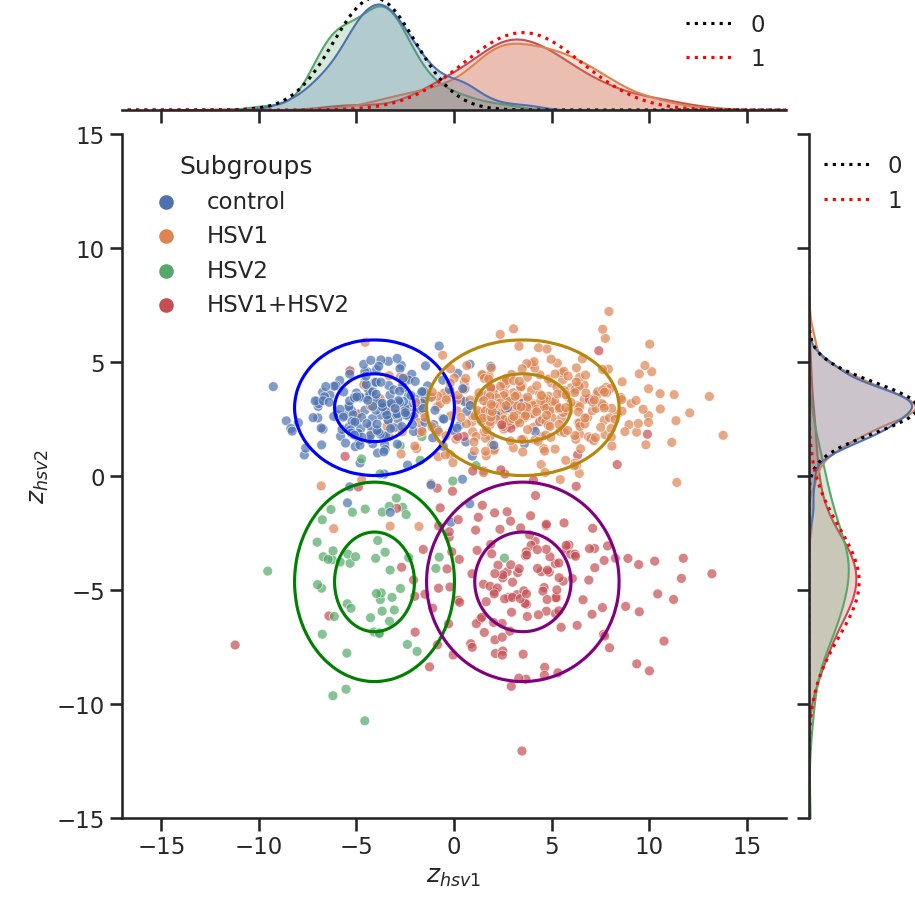}
        \caption{Train set}
	\end{minipage}
 \begin{minipage}{0.44\textwidth}
		%\includegraphics[width=\textwidth]{figures/latent_space/fig1a_annotated}
        %\includegraphics[width=\textwidth]{figures/covid/latent_covid_best.png}
        %\includegraphics[width=\textwidth]{figures/hsv12/best_run/latent_holdout.png}
        \includegraphics[width=\textwidth]{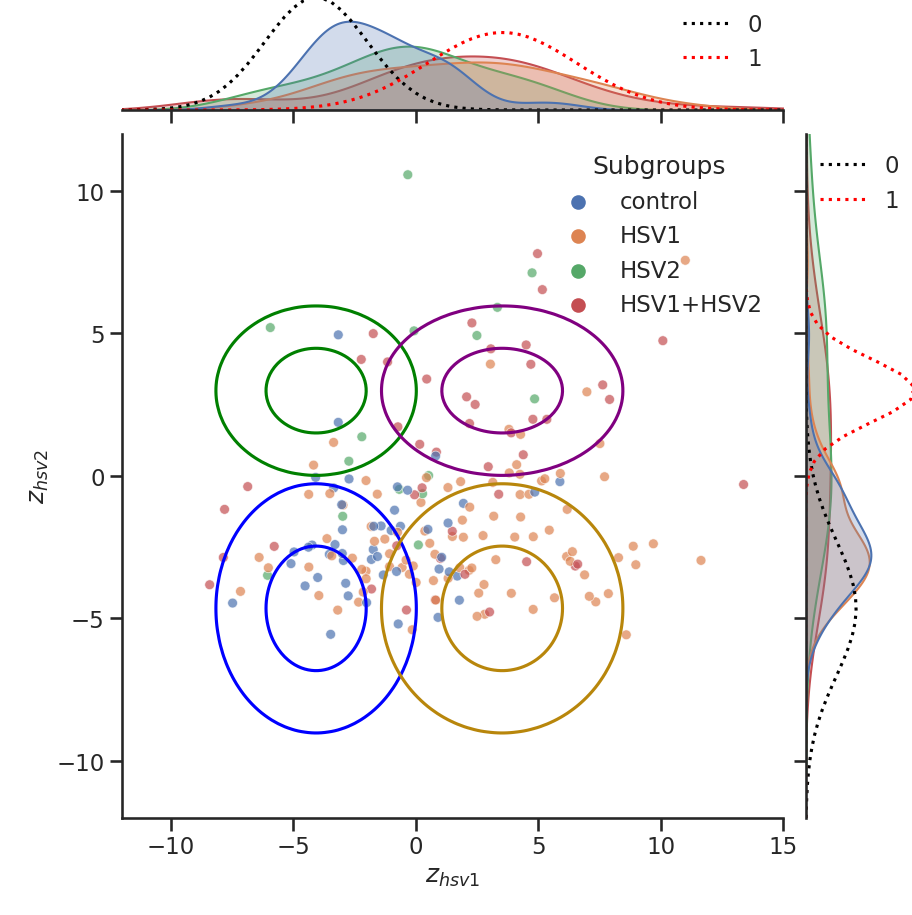}
        \caption{Holdout set}
	\end{minipage}
	\caption{\textbf{Latent space for HSV}. Each point corresponds to one sample $z$ from the posterior $q(z|x)$ in holdout. On the sides, we show marginal posterior as continuous lines, and predictive priors as dashed lines. Predictive priors $p(z_y|y)$ for each combination of labels $y$ are represented as ellipses, each circle corresponding to one standard deviation.}
	\label{fig:latent_space_hsv12}
\end{figure}
